# Supplementary material for: Xiezhi: An Ever-Updating Benchmark for Holistic Domain Knowledge Evaluation
Source: arXiv:2306.05783 source file (2024-03-11)
Supplement: Supplementary file 3 [file appendix_experiments.easy.english.tex]

\begin{table}[!t]
    \centering
    \resizebox{\textwidth}{!}{
    \begin{tabular}{c|ccc|ccc|ccc|ccc}
        \toprule
         Subjects & \multicolumn{3}{c}{bloomz-560m} & \multicolumn{3}{|c}{bloomz-1b1} & \multicolumn{3}{|c}{bloomz-1b7} & \multicolumn{3}{|c}{bloomz-3b} \\
         & 0-shot & 1-shot & 3-shot & 0-shot & 1-shot & 3-shot & 0-shot & 1-shot & 3-shot & 0-shot & 1-shot & 3-shot
         \\
        \hline
        Philosophy      & - & - & - & - & - & - & - & - & - & - & - & -  \\
        Economics       & - & - & - & - & - & - & - & - & - & - & - & -  \\
        Jurisprudence   & - & - & - & - & - & - & - & - & - & - & - & -  \\
        Pedagogy        & - & - & - & - & - & - & - & - & - & - & - & -  \\
        Literature      & - & - & - & - & - & - & - & - & - & - & - & -  \\
        History         & - & - & - & - & - & - & - & - & - & - & - & -  \\
        Science         & - & - & - & - & - & - & - & - & - & - & - & -  \\
        Engineering     & - & - & - & - & - & - & - & - & - & - & - & -  \\
        Agronomy        & - & - & - & - & - & - & - & - & - & - & - & -  \\
        Medicine        & - & - & - & - & - & - & - & - & - & - & - & -  \\
        Management      & - & - & - & - & - & - & - & - & - & - & - & -  \\
        Art Studies     & - & - & - & - & - & - & - & - & - & - & - & -  \\
        \hline
        Average         & - & - & - & - & - & - & - & - & - & - & - & -  \\
        
        \bottomrule
    \end{tabular}
    }
    \caption{Result on Xiezhi-Easy-English}
    \label{tab:detailedModelsPerformance}
\end{table}

\begin{table}[!t]
    \centering
    \resizebox{\textwidth}{!}{
    \begin{tabular}{c|ccc|ccc|ccc|ccc}
        \toprule
         Subjects & \multicolumn{3}{|c}{bloomz-7b1} & \multicolumn{3}{|c}{bloomz-7b1-mt} & \multicolumn{3}{|c}{bloomz-7b1-p3} & \multicolumn{3}{|c}{bloomz}\\
         & 0-shot & 1-shot & 3-shot & 0-shot & 1-shot & 3-shot & 0-shot & 1-shot & 3-shot & 0-shot & 1-shot & 3-shot 
         \\
        \hline
        Philosophy      & - & - & - & - & - & - & - & - & - & - & - & -  \\
        Economics       & - & - & - & - & - & - & - & - & - & - & - & -  \\
        Jurisprudence   & - & - & - & - & - & - & - & - & - & - & - & -  \\
        Pedagogy        & - & - & - & - & - & - & - & - & - & - & - & -  \\
        Literature      & - & - & - & - & - & - & - & - & - & - & - & -  \\
        History         & - & - & - & - & - & - & - & - & - & - & - & -  \\
        Science         & - & - & - & - & - & - & - & - & - & - & - & -  \\
        Engineering     & - & - & - & - & - & - & - & - & - & - & - & -  \\
        Agronomy        & - & - & - & - & - & - & - & - & - & - & - & -  \\
        Medicine        & - & - & - & - & - & - & - & - & - & - & - & -  \\
        Management      & - & - & - & - & - & - & - & - & - & - & - & -  \\
        Art Studies     & - & - & - & - & - & - & - & - & - & - & - & -  \\
        \hline
        Average         & - & - & - & - & - & - & - & - & - & - & - & -  \\
        
        \bottomrule
    \end{tabular}
    }
    \caption{Result on Xiezhi-Easy-English}
    \label{tab:detailedModelsPerformance}
\end{table}

\begin{table}[!t]
    \centering
    \resizebox{\textwidth}{!}{
    \begin{tabular}{c|ccc|ccc|ccc|ccc}
        \toprule
         Subjects & \multicolumn{3}{c}{vicuna-7B} & \multicolumn{3}{|c}{alpaca-7B} & \multicolumn{3}{c}{vicuna-13B} & \multicolumn{3}{|c}{alpaca-13B}\\
         & 0-shot & 1-shot & 3-shot & 0-shot & 1-shot & 3-shot & 0-shot & 1-shot & 3-shot & 0-shot & 1-shot & 3-shot
         \\
        \hline
        Philosophy      & - & - & - & - & - & - & - & - & - & - & - & -  \\
        Economics       & - & - & - & - & - & - & - & - & - & - & - & -  \\
        Jurisprudence   & - & - & - & - & - & - & - & - & - & - & - & -  \\
        Pedagogy        & - & - & - & - & - & - & - & - & - & - & - & -  \\
        Literature      & - & - & - & - & - & - & - & - & - & - & - & -  \\
        History         & - & - & - & - & - & - & - & - & - & - & - & -  \\
        Science         & - & - & - & - & - & - & - & - & - & - & - & -  \\
        Engineering     & - & - & - & - & - & - & - & - & - & - & - & -  \\
        Agronomy        & - & - & - & - & - & - & - & - & - & - & - & -  \\
        Medicine        & - & - & - & - & - & - & - & - & - & - & - & -  \\
        Management      & - & - & - & - & - & - & - & - & - & - & - & -  \\
        Art Studies     & - & - & - & - & - & - & - & - & - & - & - & -  \\
        \hline
        Average         & - & - & - & - & - & - & - & - & - & - & - & -  \\
        
        \bottomrule
    \end{tabular}
    }
    \caption{Result on Xiezhi-Easy-English}
    \label{tab:detailedModelsPerformance}
\end{table}


\begin{table}[!t]
    \centering
    \resizebox{\textwidth}{!}{
    \begin{tabular}{c|ccc|ccc|ccc|ccc}
        \toprule
         Subjects & \multicolumn{3}{c}{koala-13B} & \multicolumn{3}{|c}{dolly-3B} & \multicolumn{3}{c}{dolly-7B} & \multicolumn{3}{|c}{dolly-12B}\\
         & 0-shot & 1-shot & 3-shot & 0-shot & 1-shot & 3-shot & 0-shot & 1-shot & 3-shot & 0-shot & 1-shot & 3-shot
         \\
        \hline
        Philosophy      & - & - & - & - & - & - & - & - & - & - & - & -  \\
        Economics       & - & - & - & - & - & - & - & - & - & - & - & -  \\
        Jurisprudence   & - & - & - & - & - & - & - & - & - & - & - & -  \\
        Pedagogy        & - & - & - & - & - & - & - & - & - & - & - & -  \\
        Literature      & - & - & - & - & - & - & - & - & - & - & - & -  \\
        History         & - & - & - & - & - & - & - & - & - & - & - & -  \\
        Science         & - & - & - & - & - & - & - & - & - & - & - & -  \\
        Engineering     & - & - & - & - & - & - & - & - & - & - & - & -  \\
        Agronomy        & - & - & - & - & - & - & - & - & - & - & - & -  \\
        Medicine        & - & - & - & - & - & - & - & - & - & - & - & -  \\
        Management      & - & - & - & - & - & - & - & - & - & - & - & -  \\
        Art Studies     & - & - & - & - & - & - & - & - & - & - & - & -  \\
        \hline
        Average         & - & - & - & - & - & - & - & - & - & - & - & -  \\
        
        \bottomrule
    \end{tabular}
    }
    \caption{Result on Xiezhi-Easy-English}
    \label{tab:detailedModelsPerformance}
\end{table}


\begin{table}[!t]
    \centering
    \resizebox{\textwidth}{!}{
    \begin{tabular}{c|ccc|ccc|ccc|ccc}
        \toprule
         Subjects & \multicolumn{3}{c}{baize-7B-lora} & \multicolumn{3}{|c}{baize-healthcare-7B-lora} & \multicolumn{3}{|c}{baize-13B-lora} & \multicolumn{3}{|c}{baize-30B-lora}\\
         & 0-shot & 1-shot & 3-shot & 0-shot & 1-shot & 3-shot & 0-shot & 1-shot & 3-shot & 0-shot & 1-shot & 3-shot
         \\
        \hline
        Philosophy      & - & - & - & - & - & - & - & - & - & - & - & -  \\
        Economics       & - & - & - & - & - & - & - & - & - & - & - & -  \\
        Jurisprudence   & - & - & - & - & - & - & - & - & - & - & - & -  \\
        Pedagogy        & - & - & - & - & - & - & - & - & - & - & - & -  \\
        Literature      & - & - & - & - & - & - & - & - & - & - & - & -  \\
        History         & - & - & - & - & - & - & - & - & - & - & - & -  \\
        Science         & - & - & - & - & - & - & - & - & - & - & - & -  \\
        Engineering     & - & - & - & - & - & - & - & - & - & - & - & -  \\
        Agronomy        & - & - & - & - & - & - & - & - & - & - & - & -  \\
        Medicine        & - & - & - & - & - & - & - & - & - & - & - & -  \\
        Management      & - & - & - & - & - & - & - & - & - & - & - & -  \\
        Art Studies     & - & - & - & - & - & - & - & - & - & - & - & -  \\
        \hline
        Average         & - & - & - & - & - & - & - & - & - & - & - & -  \\
        
        \bottomrule
    \end{tabular}
    }
    \caption{Result on Xiezhi-Easy-English}
    \label{tab:detailedModelsPerformance}
\end{table}

\begin{table}[!t]
    \centering
    \resizebox{\textwidth}{!}{
    \begin{tabular}{c|ccc|ccc|ccc|ccc}
        \toprule
         Subjects & \multicolumn{3}{c}{belle-0.2M} & \multicolumn{3}{|c}{belle-0.6M} & \multicolumn{3}{|c}{belle-1M} & \multicolumn{3}{|c}{belle-2M}\\
         & 0-shot & 1-shot & 3-shot & 0-shot & 1-shot & 3-shot & 0-shot & 1-shot & 3-shot & 0-shot & 1-shot & 3-shot
         \\
        \hline
        Philosophy      & - & - & - & - & - & - & - & - & - & - & - & -  \\
        Economics       & - & - & - & - & - & - & - & - & - & - & - & -  \\
        Jurisprudence   & - & - & - & - & - & - & - & - & - & - & - & -  \\
        Pedagogy        & - & - & - & - & - & - & - & - & - & - & - & -  \\
        Literature      & - & - & - & - & - & - & - & - & - & - & - & -  \\
        History         & - & - & - & - & - & - & - & - & - & - & - & -  \\
        Science         & - & - & - & - & - & - & - & - & - & - & - & -  \\
        Engineering     & - & - & - & - & - & - & - & - & - & - & - & -  \\
        Agronomy        & - & - & - & - & - & - & - & - & - & - & - & -  \\
        Medicine        & - & - & - & - & - & - & - & - & - & - & - & -  \\
        Management      & - & - & - & - & - & - & - & - & - & - & - & -  \\
        Art Studies     & - & - & - & - & - & - & - & - & - & - & - & -  \\
        \hline
        Average         & - & - & - & - & - & - & - & - & - & - & - & -  \\
        
        \bottomrule
    \end{tabular}
    }
    \caption{Result on Xiezhi-Easy-English}
    \label{tab:detailedModelsPerformance}
\end{table}


\begin{table}[!t]
    \centering
    \resizebox{\textwidth}{!}{
    \begin{tabular}{c|ccc|ccc|ccc|ccc}
        \toprule
         Subjects & \multicolumn{3}{c}{gpt-neox-20B} & \multicolumn{3}{|c}{h2ogpt-12B} & \multicolumn{3}{|c}{h2ogpt-20B} & \multicolumn{3}{|c}{h2ogpt-20B-mutilang}\\
         & 0-shot & 1-shot & 3-shot & 0-shot & 1-shot & 3-shot & 0-shot & 1-shot & 3-shot & 0-shot & 1-shot & 3-shot
         \\
        \hline
        Philosophy      & - & - & - & - & - & - & - & - & - & - & - & -  \\
        Economics       & - & - & - & - & - & - & - & - & - & - & - & -  \\
        Jurisprudence   & - & - & - & - & - & - & - & - & - & - & - & -  \\
        Pedagogy        & - & - & - & - & - & - & - & - & - & - & - & -  \\
        Literature      & - & - & - & - & - & - & - & - & - & - & - & -  \\
        History         & - & - & - & - & - & - & - & - & - & - & - & -  \\
        Science         & - & - & - & - & - & - & - & - & - & - & - & -  \\
        Engineering     & - & - & - & - & - & - & - & - & - & - & - & -  \\
        Agronomy        & - & - & - & - & - & - & - & - & - & - & - & -  \\
        Medicine        & - & - & - & - & - & - & - & - & - & - & - & -  \\
        Management      & - & - & - & - & - & - & - & - & - & - & - & -  \\
        Art Studies     & - & - & - & - & - & - & - & - & - & - & - & -  \\
        \hline
        Average         & - & - & - & - & - & - & - & - & - & - & - & -  \\
        
        \bottomrule
    \end{tabular}
    }
    \caption{Result on Xiezhi-Easy-English}
    \label{tab:detailedModelsPerformance}
\end{table}

\begin{table}[!t]
    \centering
    \resizebox{\textwidth}{!}{
    \begin{tabular}{c|ccc|ccc|ccc|ccc}
        \toprule
         Subjects & \multicolumn{3}{|c}{ChatGLM-6B} & \multicolumn{3}{|c}{DoctorGLM-6B} & \multicolumn{3}{|c}{Med-ChatGLM-6B} & \multicolumn{3}{|c}{LawGPT-6B}\\
         & 0-shot & 1-shot & 3-shot & 0-shot & 1-shot & 3-shot & 0-shot & 1-shot & 3-shot & 0-shot & 1-shot & 3-shot 
         \\
        \hline
        Philosophy      & - & - & - & - & - & - & - & - & - & - & - & -  \\
        Economics       & - & - & - & - & - & - & - & - & - & - & - & -  \\
        Jurisprudence   & - & - & - & - & - & - & - & - & - & - & - & -  \\
        Pedagogy        & - & - & - & - & - & - & - & - & - & - & - & -  \\
        Literature      & - & - & - & - & - & - & - & - & - & - & - & -  \\
        History         & - & - & - & - & - & - & - & - & - & - & - & -  \\
        Science         & - & - & - & - & - & - & - & - & - & - & - & -  \\
        Engineering     & - & - & - & - & - & - & - & - & - & - & - & -  \\
        Agronomy        & - & - & - & - & - & - & - & - & - & - & - & -  \\
        Medicine        & - & - & - & - & - & - & - & - & - & - & - & -  \\
        Management      & - & - & - & - & - & - & - & - & - & - & - & -  \\
        Art Studies     & - & - & - & - & - & - & - & - & - & - & - & -  \\
        \hline
        Average         & - & - & - & - & - & - & - & - & - & - & - & -  \\
        \bottomrule
    \end{tabular}
    }
    \caption{Result on Xiezhi-Easy-English}
    \label{tab:detailedModelsPerformance}
\end{table}


\begin{table}[!t]
    \centering
    \resizebox{\textwidth}{!}{
    \begin{tabular}{c|ccc|ccc|ccc|ccc}
        \toprule
         Subjects & \multicolumn{3}{|c}{moss-base-16B} & \multicolumn{3}{|c}{moss-sft-16B} & \multicolumn{3}{|c}{stablelm-7B} & \multicolumn{3}{|c}{stablelm-13B}\\
         & 0-shot & 1-shot & 3-shot & 0-shot & 1-shot & 3-shot & 0-shot & 1-shot & 3-shot & 0-shot & 1-shot & 3-shot 
         \\
        \hline
        Philosophy      & - & - & - & - & - & - & - & - & - & - & - & -  \\
        Economics       & - & - & - & - & - & - & - & - & - & - & - & -  \\
        Jurisprudence   & - & - & - & - & - & - & - & - & - & - & - & -  \\
        Pedagogy        & - & - & - & - & - & - & - & - & - & - & - & -  \\
        Literature      & - & - & - & - & - & - & - & - & - & - & - & -  \\
        History         & - & - & - & - & - & - & - & - & - & - & - & -  \\
        Science         & - & - & - & - & - & - & - & - & - & - & - & -  \\
        Engineering     & - & - & - & - & - & - & - & - & - & - & - & -  \\
        Agronomy        & - & - & - & - & - & - & - & - & - & - & - & -  \\
        Medicine        & - & - & - & - & - & - & - & - & - & - & - & -  \\
        Management      & - & - & - & - & - & - & - & - & - & - & - & -  \\
        Art Studies     & - & - & - & - & - & - & - & - & - & - & - & -  \\
        \hline
        Average         & - & - & - & - & - & - & - & - & - & - & - & -  \\
        \bottomrule
    \end{tabular}
    }
    \caption{Result on Xiezhi-Easy-English}
    \label{tab:detailedModelsPerformance}
\end{table}


\begin{table}[!t]
    \centering
    \resizebox{\textwidth}{!}{
    \begin{tabular}{c|ccc|ccc|ccc|ccc}
        \toprule
         Subjects & \multicolumn{3}{|c}{pythia-1.4B} & \multicolumn{3}{|c}{pythia-2.8B} & \multicolumn{3}{|c}{pythia-6.9B} & \multicolumn{3}{|c}{pythia-12B}\\
         & 0-shot & 1-shot & 3-shot & 0-shot & 1-shot & 3-shot & 0-shot & 1-shot & 3-shot & 0-shot & 1-shot & 3-shot 
         \\
        \hline
        Philosophy      & - & - & - & - & - & - & - & - & - & - & - & -  \\
        Economics       & - & - & - & - & - & - & - & - & - & - & - & -  \\
        Jurisprudence   & - & - & - & - & - & - & - & - & - & - & - & -  \\
        Pedagogy        & - & - & - & - & - & - & - & - & - & - & - & -  \\
        Literature      & - & - & - & - & - & - & - & - & - & - & - & -  \\
        History         & - & - & - & - & - & - & - & - & - & - & - & -  \\
        Science         & - & - & - & - & - & - & - & - & - & - & - & -  \\
        Engineering     & - & - & - & - & - & - & - & - & - & - & - & -  \\
        Agronomy        & - & - & - & - & - & - & - & - & - & - & - & -  \\
        Medicine        & - & - & - & - & - & - & - & - & - & - & - & -  \\
        Management      & - & - & - & - & - & - & - & - & - & - & - & -  \\
        Art Studies     & - & - & - & - & - & - & - & - & - & - & - & -  \\
        \hline
        Average         & - & - & - & - & - & - & - & - & - & - & - & -  \\
        \bottomrule
    \end{tabular}
    }
    \caption{Result on Xiezhi-Easy-English}
    \label{tab:detailedModelsPerformance}
\end{table}

\begin{table}[!t]
    \centering
    \resizebox{\textwidth}{!}{
    \begin{tabular}{c|ccc|ccc|ccc|ccc}
        \toprule
         Subjects & \multicolumn{3}{|c}{llama-7B} & \multicolumn{3}{|c}{llama-13B} & \multicolumn{3}{|c}{llama-30B} & \multicolumn{3}{|c}{llama-65B}\\
         & 0-shot & 1-shot & 3-shot & 0-shot & 1-shot & 3-shot & 0-shot & 1-shot & 3-shot & 0-shot & 1-shot & 3-shot 
         \\
        \hline
        Philosophy      & - & - & - & - & - & - & - & - & - & - & - & -  \\
        Economics       & - & - & - & - & - & - & - & - & - & - & - & -  \\
        Jurisprudence   & - & - & - & - & - & - & - & - & - & - & - & -  \\
        Pedagogy        & - & - & - & - & - & - & - & - & - & - & - & -  \\
        Literature      & - & - & - & - & - & - & - & - & - & - & - & -  \\
        History         & - & - & - & - & - & - & - & - & - & - & - & -  \\
        Science         & - & - & - & - & - & - & - & - & - & - & - & -  \\
        Engineering     & - & - & - & - & - & - & - & - & - & - & - & -  \\
        Agronomy        & - & - & - & - & - & - & - & - & - & - & - & -  \\
        Medicine        & - & - & - & - & - & - & - & - & - & - & - & -  \\
        Management      & - & - & - & - & - & - & - & - & - & - & - & -  \\
        Art Studies     & - & - & - & - & - & - & - & - & - & - & - & -  \\
        \hline
        Average         & - & - & - & - & - & - & - & - & - & - & - & -  \\
        \bottomrule
    \end{tabular}
    }
    \caption{Result on Xiezhi-Easy-English}
    \label{tab:detailedModelsPerformance}
\end{table}


\begin{table}[!t]
    \centering
    \resizebox{\textwidth}{!}{
    \begin{tabular}{c|ccc|ccc|ccc|ccc|ccc}
        \toprule
         Subjects & \multicolumn{3}{c}{GPT-4} & \multicolumn{3}{|c}{ChatGPT} & \multicolumn{3}{|c}{ChatGLM-130B} & \multicolumn{3}{|c}{Xinghuo}\\
         & 0-shot & 1-shot & 3-shot & 0-shot & 1-shot & 3-shot & 0-shot & 1-shot & 3-shot & 0-shot & 1-shot & 3-shot 
         \\
        \hline
        Philosophy      & - & - & - & - & - & - & - & - & - & - & - & -  \\
        Economics       & - & - & - & - & - & - & - & - & - & - & - & -  \\
        Jurisprudence   & - & - & - & - & - & - & - & - & - & - & - & -  \\
        Pedagogy        & - & - & - & - & - & - & - & - & - & - & - & -  \\
        Literature      & - & - & - & - & - & - & - & - & - & - & - & -  \\
        History         & - & - & - & - & - & - & - & - & - & - & - & -  \\
        Science         & - & - & - & - & - & - & - & - & - & - & - & -  \\
        Engineering     & - & - & - & - & - & - & - & - & - & - & - & -  \\
        Agronomy        & - & - & - & - & - & - & - & - & - & - & - & -  \\
        Medicine        & - & - & - & - & - & - & - & - & - & - & - & -  \\
        Management      & - & - & - & - & - & - & - & - & - & - & - & -  \\
        Art Studies     & - & - & - & - & - & - & - & - & - & - & - & -  \\
        \hline
        Average         & - & - & - & - & - & - & - & - & - & - & - & -  \\
        \bottomrule
    \end{tabular}
    }
    \caption{Result on Xiezhi-Easy-English}
    \label{tab:detailedModelsPerformance}
\end{table}
